# Supplementary material for: Learning to Bid Long-Term: Multi-Agent Reinforcement Learning with Long-Term and Sparse Reward in Repeated Auction Games
Source: arXiv:2204.02268 source file (2022-04-05)
Supplement: Supplementary file 1 [file appendix.tex]

\appendices
\section{Proof of potential game}
\label{appendix:potentialGame}

\begin{proof} 

We define player $i$'s utility as $u_i(\alpha_i,\alpha_{-i})=\sum\limits_{k \in K}q_{i,k}-\sum\limits_{k \in K}\alpha_{i,k} q_{i,k} + W \Big(1-\frac{\sum_j \alpha_j \cdot \omega_j}{C}\Big)$, where $\omega_j \in \mathbb{R}^K$ is the resource requirement of each commodity, $C$ is the system capacity. 

We define potential function: $\phi(\alpha_i,\alpha_{-i})=\sum\limits_{j \in I, k \in K}q_{j,k}-\sum\limits_{j \in I, k \in K} \alpha_{j,k}q_{j,k}+W\Big(1-\frac{\sum_j \alpha_j \cdot \omega_j}{C} \Big)$. 

To simplify, we substitute with $Q_i=\sum\limits_{k\in K}q_{i,k}$, $A_i=\sum\limits_{k \in K}\alpha_{i,k} q_{i,k}$, $A_{-i} = \sum\limits_{j \in I, j \neq i, k \in K}\alpha_{j,k} q_{j,k}$, $B_i=\sum\limits_k \alpha_{i,k} \omega_{i,k}$, $B_{-i}=\sum\limits_{j \in I, j \neq i, k \in K}\alpha_{j,k} \omega_{j,k}$, and rewrite: $u_i(\alpha_i,\alpha_{-i})=Q_i-A_i+W-\frac{W}{C}(B_i+B_{-i})$ and $u_i(\alpha'_i,\alpha_{-i})=Q_i-A'_i+W-\frac{W}{C}(B'_i+B_{-i})$; hence, $\phi(\alpha_i,\alpha_{-i}) = \sum\limits_j Q_j-(A_i+A_{-i})+W-\frac{W(B_i+B_{-i})}{C}$, $\phi(\alpha'_i,\alpha_{-i}) = \sum\limits_j Q_j-(A'_i+A_{-i})+W-\frac{W(B'_i+B_{-i}) }{C}$, which implies $u_i(\alpha_i,\alpha_{-i})-u_i(\alpha'_i,\alpha_{-i}) =-(A_i-A'_i)-\frac{W}{C}(B_i-B'_i) =\phi(\alpha_i,\alpha_{-i})-\phi(\alpha'_i,\alpha_{-i})$. %Since $\alpha_i \in \mathbb R^{|K|}$, the game under low contention is a finite potential game.
\end{proof}

\section{Second-price auction}
\label{appendix:SPAwithpenalty}
Under high contention, as defined in Sec.\ref{payment}, $u_i$ is reduced to: \begin{flalign}\label{eq:ui}
u_i= \sum\limits_{k \in K} \Big(x_{i,k} \cdot (v_{i,k}-p_{i,k})-(1-x_{i,k}) \cdot c_{i,k} \Big)
\end{flalign}

We prove the theorem for $|M|=2$ and $|K|=1$, extension to other settings is straightforward. Our proof is an extension from \cite{sun2006wireless}. Unlike \cite{sun2006wireless}, we include in utility the second-price payment and cost for losing a bid. Based on \cite{sun2006wireless}, it can also be extended to multiple bidders. %We also prove more formally the conditions to apply Kakutani fixed point theorem, as an extention to \cite{sun2006wireless}.

$2$ bidders receive continuously distributed valuations $v_i \in [l_i,m_i], i \in\{1,2\}$ for $1$ commodity, and choose their strategies $f_1(v_1),f_2(v_2)$ from the strategy sets $F_1$ and $F_2$. The resulting NE strategy pair is $(f_1^*, f_2^*)$. Any strategy function $f(v)$ is increasing in $v$, with $f_1(l_1)=a$, and $f_1(m_1)=b$. We assume users have budgets $(B_1,B_2)$, and that they cannot bid more than the budget. We define cost for losing the bid $c_i$.

We formulate the problem into a utility maximization problem: $\max\limits_{f_2 \in S_2(f_1)} u_2(f_1,f_2)$. We say $f_2$ is a best response of bidder 2, if $u_2(f_1,f_2)\geq u_2(f_1,f_2')$, $\forall f_2' \in S_2(f_1)$. A NE strategy pair $(f_1^*, f_2^*)$ has the strategies as each other's best responses. 

\begin{thm}\label{thm:bestResp} Given bidder 1's bidding strategy $f_1 \in F_1,f_1(l_1)=a_1,f_1(m_1)=b_1$, bidder 2's best response has the form $\begin{cases}
f_2(v_2) \leq a_1 & \text{for } v_2 \in [l_2,\theta_1] \\
f_2(v_2) = j_2 \cdot v_2 + d_2& \text{for } v_2 \in [\theta_1,\theta_2] \\
f_2(v_2) \geq b_1 & \text{for } v_2 \in [\theta_2,m_2]
\end{cases}$, where $\theta_1, \theta_2 \in [l_2,m_2]$ and $j_2 \theta_1 + d_2 =a_1, j_2\theta_2 + d_2 =b_1$.
\end{thm}

Theorem \ref{thm:bestResp} implies that the best response of bidder $1$ and $2$ are both of the linear form. Using the new best responses function, we similarly extend the proof of the NE outcome and welfare maximization to suit our case. Detailed proof is provided in supplemental meterial \cite{dracosource}.

\section{Pareto optimality}
\label{appendix:paretoOptimal}

Valuation of the service request is a linear function of the resource needed: $v_1=g_1 \omega_1 + k_1,v_2=g_2 \omega_2+k_2$, $g,k$ are constants, $\omega$ is amount of resource required. The allocation rule under NE is: $A^*_{v_1,v_2}=1 \text{, if } j_1 v_1 + d_1 \geq j_2 v_2 + d_2 \text{, otherwise } 2$. Form of the condition is from best response form in appendix Sec.\ref{appendix:SPAwithpenalty}. We also assume that both bidders have at least some access to the resources, as a form of fairness. We define the fairness constraint: $\mathbb{E}[\omega_1|_{A_{v1,v2}=1}] / \mathbb{E}[\omega_2|_{A_{v1,v2}=2}]=\gamma \in \mathbb R_{>0}$.

\begin{thm}
The allocation $A^*_{v_1,v_2}$ maximizes overall resource allocation $\omega_1+\omega_2$, subject to the fairness constraint, when the valuations are linear functions of resources. Or, the NE of the game achieves optimal resource allocation.
\end{thm}

\begin{proof}
Find the Lagrangian multiplier $\lambda^*$ that satisfies the fairness constraint with NE allocation $A^*_{v_1,v_2}$. Define $g,k$ as: $g_1 = (1+\lambda^*)/j_1 \text{ , } k_1 =-d_1/j_1$, and $g_2 = (1-\gamma \lambda^*)/j_2 \text{ , } k_2 =-d_2/j_2$. We rewrite the allocation: $A^*_{\omega_1,\omega_2} = 1 \text{, if } \omega_1 (1+\lambda^*) \geq \omega_2(1-\gamma \lambda^*) \text{, otherwise } 2$. Rest of the proof is same as \cite{sun2006wireless}.
\end{proof}
